# Supplementary material for: Bridging Local and Global Knowledge via Transformer in Board Games
Source: arXiv:2410.05347 source file (2025-07-18)
Supplement: Supplementary file 3 [file 11.tex]

\renewcommand{\patternNum}{11}
\begin{figure*}[t]
\centering
\resizebox{0.9\columnwidth}{!}{
\subfloat[ID-\patternNum]{\includegraphics[width=0.24\columnwidth]{figures/Appendix/mark_X/\patternNum.pdf}\label{fig:label_position_\patternNum}}
\hspace{0.005\columnwidth}
\subfloat[Ground truth]{\includegraphics[width=0.24\columnwidth]{figures/Appendix/ground_truth/\patternNum.pdf}\label{fig:ground_truth_\patternNum}}
% \
\hspace{0.005\columnwidth}
\subfloat[\texttt{10R}]{\includegraphics[width=0.24\columnwidth]{figures/Appendix/10R/\patternNum.pdf}\label{fig:10R_pattern_\patternNum a}}
\hspace{0.005\columnwidth}
\subfloat[\texttt{R3(RRT)}]{\includegraphics[width=0.24\columnwidth]{figures/Appendix/10RT/\patternNum.pdf}\label{fig:10RT_pattern_\patternNum a}}
}
\caption{Circular pattern \patternNum.}
\label{fig:10R_10RT_pattern_\patternNum}
\end{figure*}
