# Supplementary material for: Bridging Local and Global Knowledge via Transformer in Board Games
Source: arXiv:2410.05347 source file (2025-07-18)

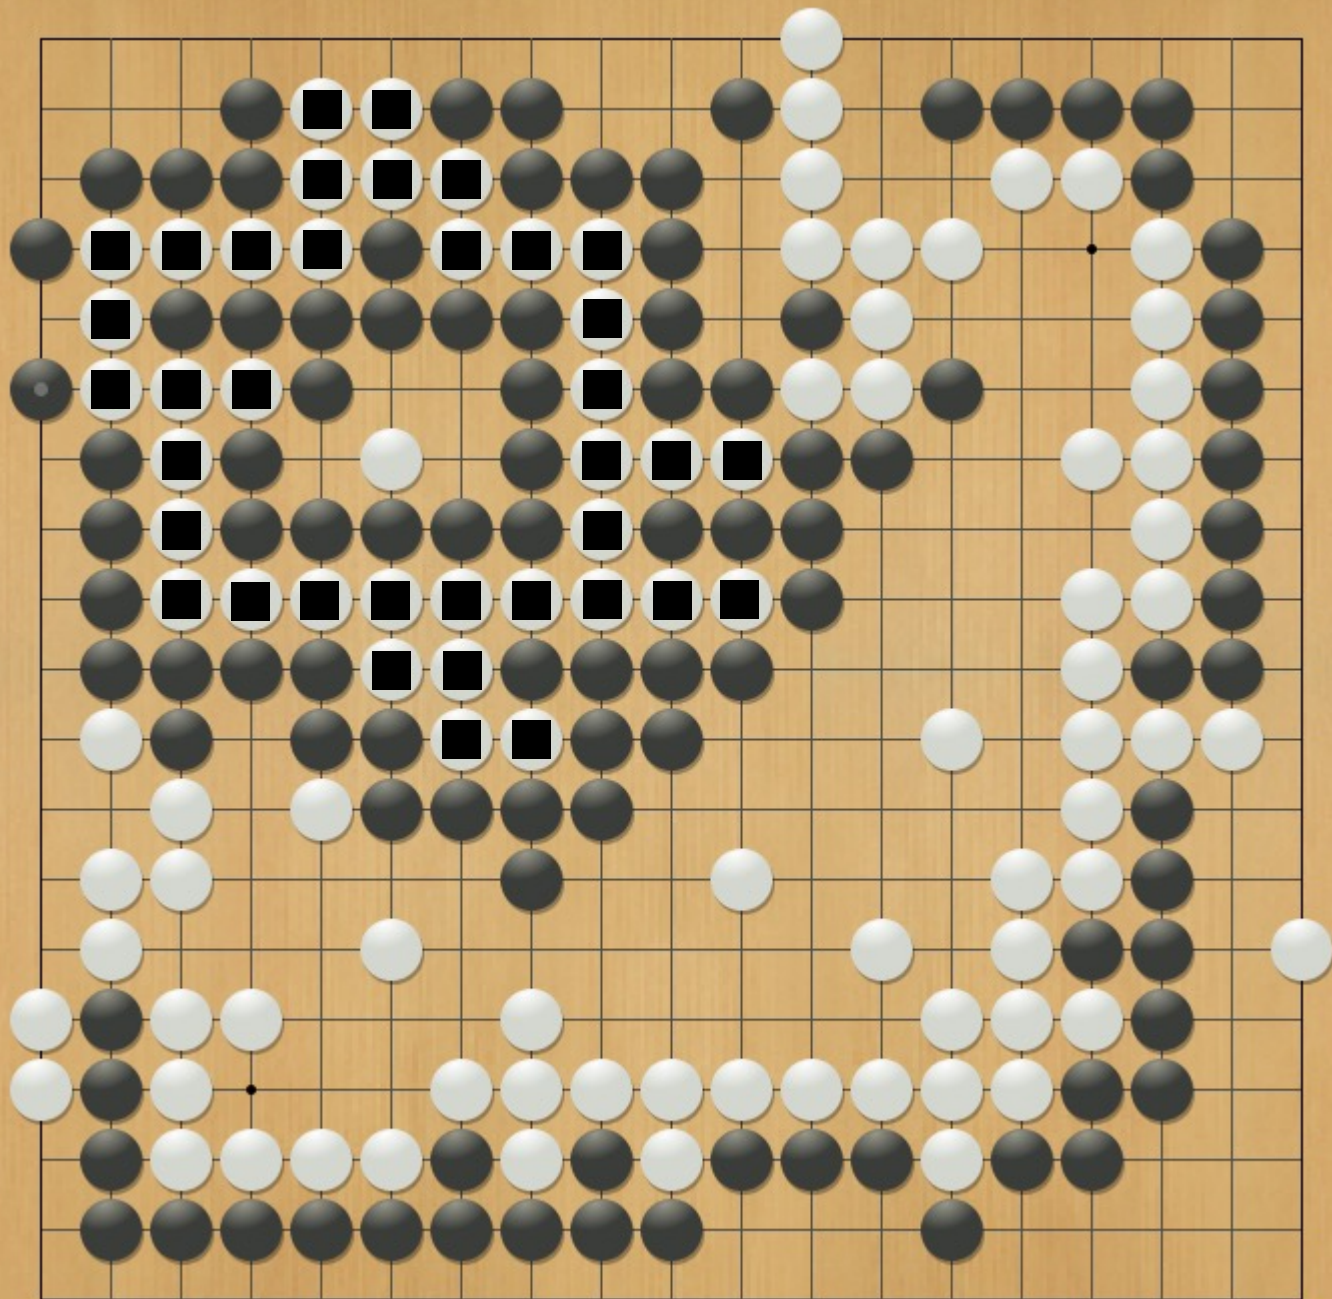

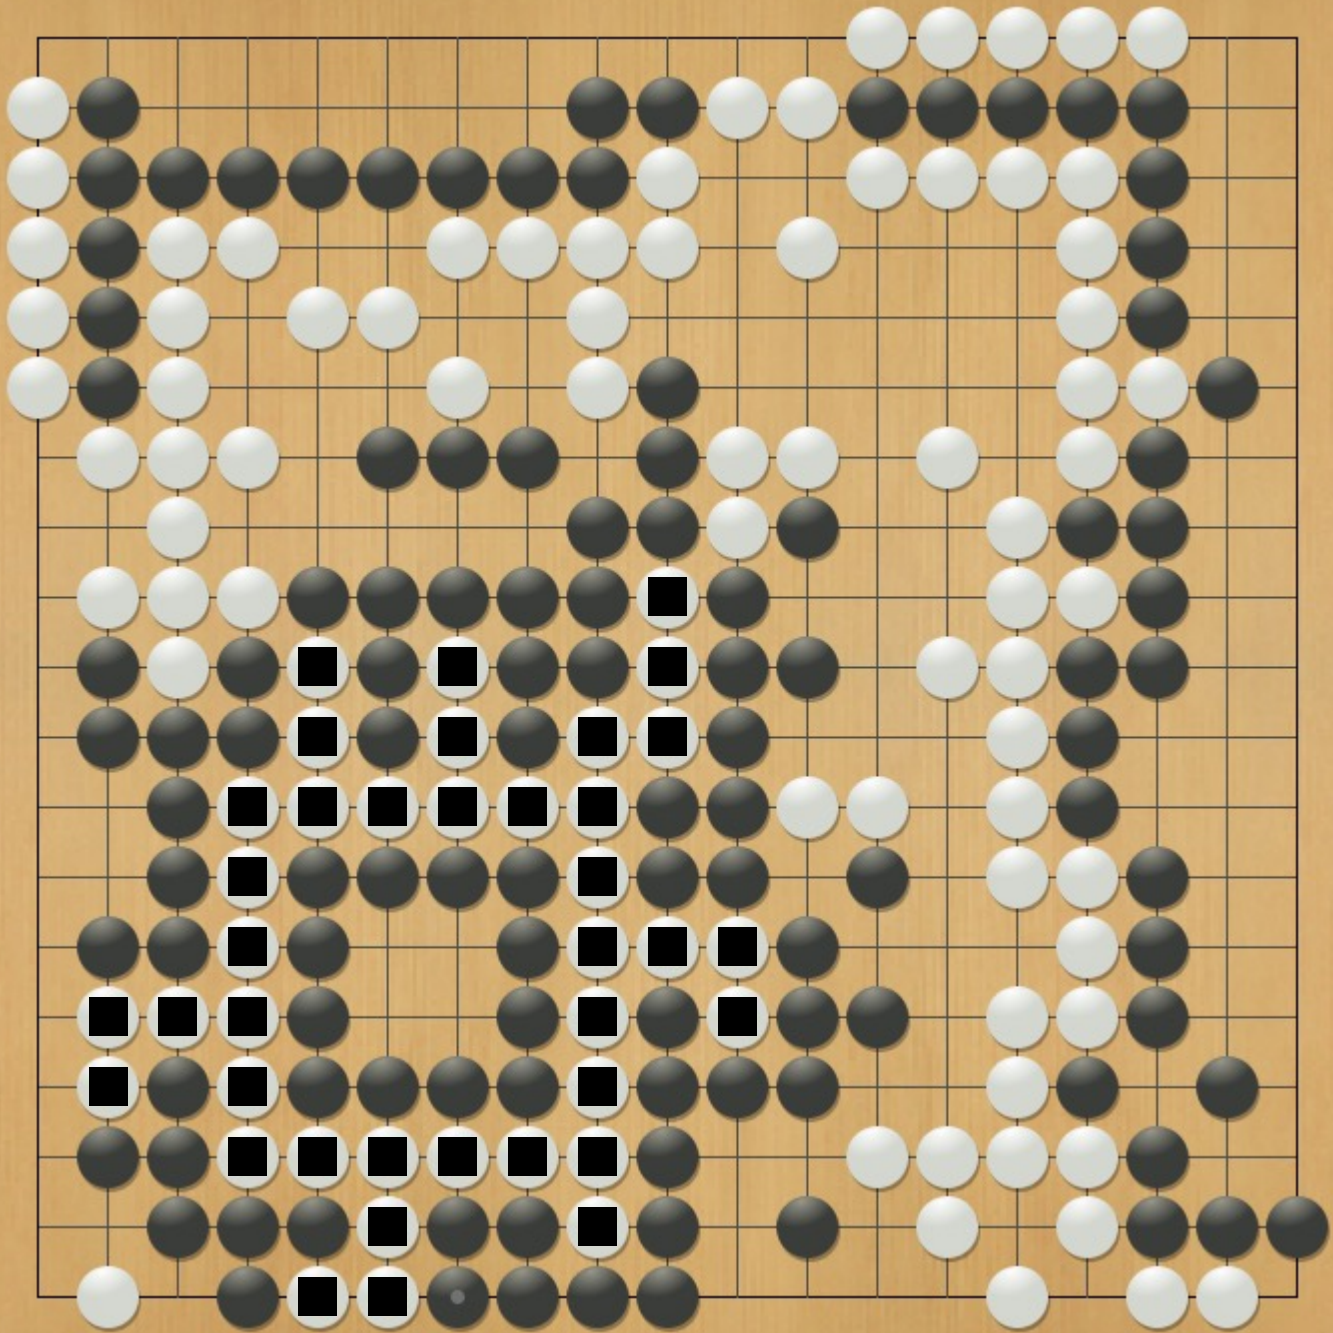

Supplement: Supplementary file 25 [file 1.pdf]
